# Supplementary material for: BiaScope: Visual Unfairness Diagnosis for Graph Embeddings
Source: arXiv:2210.06417 source file (2022-10-12)
Supplement: Supplementary file 1 [file supplemental.tex]

\newpage
\appendix

\section{Detailed Task Analysis}

\begin{table*}[ht]
\centering
\caption{Based on our interview with Professor Tina Eliassi-Rad we extracted the tasks described in the table. For each domain task on the left, we provide an example and then we list the high, mid, and low level abstract tasks \cite{munzner2014visualization, amar2005low} along with the graph-specific abstract task \cite{lee2006task}.  The domain tasks are listed in order of priority. }
\label{tab:tasks_full}
\begin{tabular}{|p{0.2\linewidth}|p{0.3\linewidth}|p{0.1\linewidth}|p{0.1\linewidth}|p{0.1\linewidth}||p{0.1\linewidth}|}
\toprule
\multicolumn{2}{|c|}{\textbf{Domain Tasks}} & \multicolumn{4}{|c|}{\textbf{Abstract Tasks}}\\ \hline
Task & Example and Description & High & Mid & Low & Graph-Specific \\\hline

\textbf{Statistical Summary} & Degree distribution, avg. degree, clustering coefficient, triangle count & Derive & Explore & Characterize Distribution & Overview \\\hline

\textbf{Embedding Comparison \textit{w.r.t.} Fairness} & Compare two embeddings w.r.t. a fairness score per node, per topological community or for the whole graph & Present & Explore & Correlate & Overview \\\hline

\textbf{Unfairness Diagnostics} & For a given embedding, find which nodes contribute to unfairness and why & Discover & Locate & Find Anomalies & Attribute-based: On the Nodes\\\hline
\\\hline
Community Detection & Separating the graph into groups & Derive & Explore & Cluster & Topology: Find Clusters \\\hline

Community Labeling & Labeling detected communities (e.g., by political party) & Annotate & Browse & Compute Derived Value & Attribute-based: On the Nodes \\\hline

Fairness Definitions Comparison & Individual vs. Group fairness: determining the impact of the fairness definition on the embedding location for a set of nodes. & Present & Browse & Correlate & Attribute-based: On the Nodes\\\hline

Set Hyperparameter Values for Fairness Definition & Determining the impact of hyperparameters on the fairness score for a set of nodes, for a given fairness definition. & Discover & Explore & Correlate & Attribute-based: On the Nodes\\\hline

Check for Representation Stability & Re-running the algorithm multiple times. & Present & Lookup & Cluster & Overview\\\hline

Disentangling Features from Topology & In a social network: visualize info from a users profile vs unified info from their friend group & Discover & Locate & Correlate & Attribute-based: On the Nodes\\\hline

Filter Graph & Filter nodes/edges e.g. filter all of the female nodes in a social network & Discover & Locate & Filter & Attribute-based: On the Nodes \\\hline

Manipulate Graph & Adding edges between nodes with common neighbors (triadic closure) & Derive & Lookup & Compute Derived Value  &  Topology: Accessibility\\\hline

Tracking Dynamic Processes & Message Passing (spread of information e.g. influence maximization and spread of disease) & Discover & Locate & Correlate & Overview\\\hline

Outlier Detection & Fraud detection & Discover & Locate & Find Anomalies & Overview\\\hline

\bottomrule
\end{tabular}
\end{table*}

In this section we provide the full task analysis we conducted after interviewing our expert. From the set of tasks analysed and categorized in Table \ref{tab:tasks_full} we identified the most important tasks our tool supports.

\section{Fairness definitions and examples}\label{sec:fairness_defs}

\subsection{Score 1: InFoRM (Individual Fairness)}

Let $Y$ be the embedding matrix, where $Y[u]$ is the embedding of node $u$. Let $S$ be the node proximity matrix, where $S[u,v]$ is the proximity of nodes $u$ and $v$. The most obvious notion of node proximity is the adjacency matrix $S=A$. There are other options such as a random walk matrix. We can then define the first individual fairness score based on \cite{InFoRM} as follows:

\begin{align*}
    score_1(u,k=1) &= \sum_{v \neq u} \lVert Y[u] - Y[v]\rVert_2^2 \cdot S[u,v] \\
    &= \sum_{v\in\mathcal{N}(u,1)} \lVert Y[u] - Y[v]\rVert_2^2
\end{align*}
where $\mathcal{N}(u,k)$ is the $k$-hop neighborhood of $u$, given by the nodes reachable from $u$ in at most $k$ steps.
We generalize this notion for different values of $k$ as follows:
\begin{align*}
    score_1(u,k) &= \sum_{v\in\mathcal{N}(u,k)} \lVert Y[u] - Y[v]\rVert_2^2
\end{align*}

\subsection{Fairwalk (Group Fairness)}

For the group fairness notions introduced in \cite{ijcai2019-456}, given a node $u$, we need to define a group of ``recommended" nodes, denoted $\rho(u)$. Among the nodes not connected to $u$, we choose to ``recommend" the top-$k$ most proximal ones in the embedding, using dot product similarity.
% \note{BS:I think the expression is wrong, change it to a new version}
% $$
% \text{\note{(wrong)}} \rho(u) = \{v \;:\; u\neq v \wedge (u,v)\not\in E \wedge v\in \texttt{top}_k(Y[u] \cdot Y[v])\}
% $$
% \note{BS:We should specify in the arg that we are talking about v only, maybe just define it in natural language}
% \begin{align*}
%     \rho(u) &= \texttt{top}_k(Y[u],\cdot) = \arg \texttt{top}_k(\{\langle Y[u],Y[v]\rangle : u\neq v \wedge (u,v)\not\in E\})
% \end{align*}
% \note{BS: If we assume we don't have self loops in the graph, we can drop $u\neq v$.}

Additionally, given a sensitive attribute $S$ and a value $z$, we can restrict the ``recommended" node set based on the attribute as follows:    
\begin{align*}
    % \rho_z(u) &=  \{v \;:\; u\neq v \wedge (u,v)\not\in E \wedge \texttt{top}_k(Y[u] \cdot Y[v]) \wedge \texttt{attr}_S(v)=z \}\\
    \rho_z(u) &= \{v \;:\; v\in\rho(u) \wedge \texttt{attr}_S(v)=z\}
\end{align*}
For example, we can have $S=\text{gender}$ and $z=\text{female}$. When computing $\rho(u)$, a criteria is needed for breaking ties in the ranking, for instance one can take smallest id goes first. Using this notions, two fairness notions are defined in \cite{ijcai2019-456}, which are described next.

\subsubsection{Network Level}

Given a sensitive attribute $S$, we can consider different communities (user groups) in the graph, according to the values of $S$. Concretely, given $i,j$ two possible values for attribute $S$, we define the group $G_{i,j}^S$ as follows:
% \note{BS: should we add $u\neq v$?}
\[
G_{i,j}^S = \{(u,v)\ : u\neq v \wedge \texttt{attr}_S(u)=i \wedge \texttt{attr}_S(u)=j\}
\]
We denote the set of all such groups as $\mathcal{G}^S$. Then,  based on these groups, a bias score can be derived as follows:

\begin{equation}
    \texttt{bias}(\mathcal{G}^S) = Var(\{P(G_{i,j}^S): G_{i,j} \in \mathcal{G}^S\})
\end{equation}
, where 
\begin{equation}
    P(G_{i,j}^S) = \frac{|\{(u,v): v \in \rho(u) \wedge (u,v) \in G_{i,j}^S\} |}{|G_{i,j}^S|} .
\end{equation}

\noindent
Example:

Let $k=1$, $S=\text{race}$ with possible attribute values $\{\text{w}, \text{b}\}$. Consider the network and associated embedding shown in Figure \ref{fig:ex_1}. 

\begin{figure}
    \centering
    \includegraphics[scale=0.3]{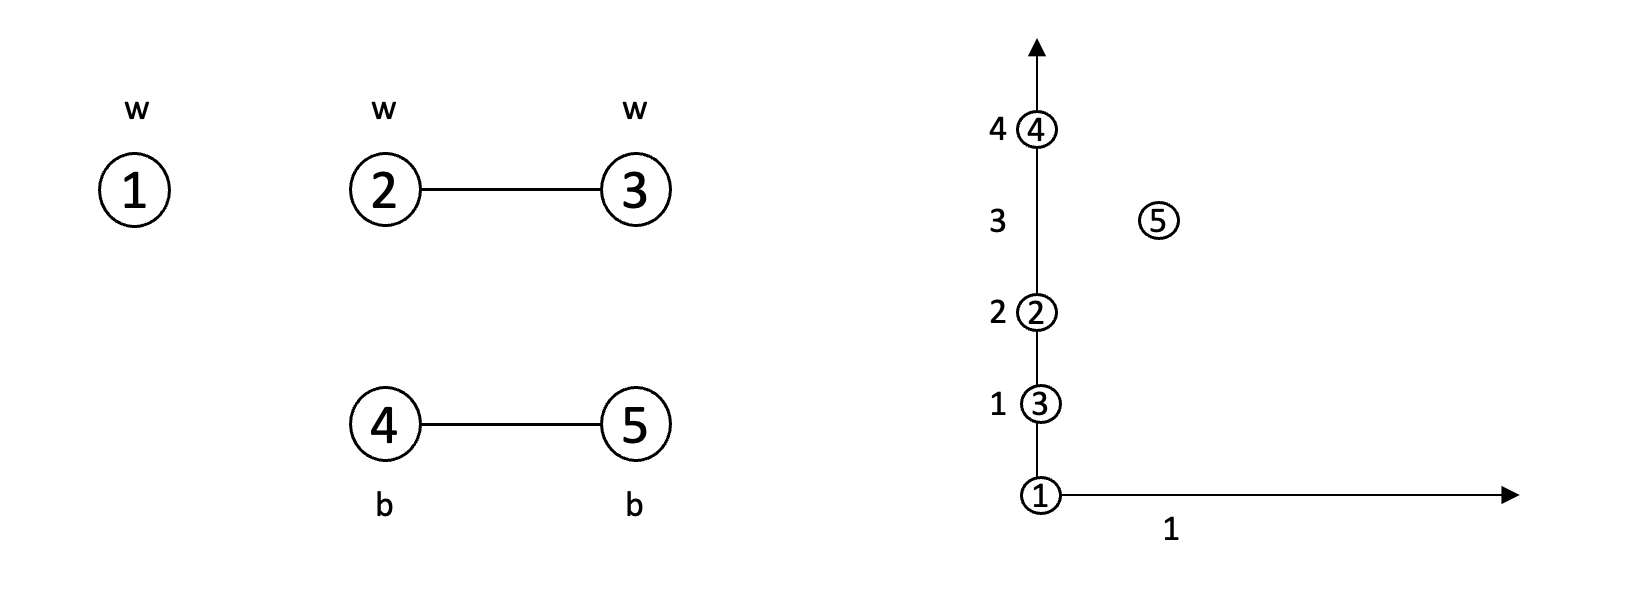}
    \caption{Example network and embedding. Race feature of the nodes is indicated next to them in the network.}
    \label{fig:ex_1}
\end{figure}

Then, we have:
\begin{align*}
    \mathcal{G}^S &= \{G^S_{w,b},G^S_{w,w},G^S_{b,b}\}\\
    G^S_{w,b} &= \{(1,4),(1,5),(2,4),(2,5),(3,4),(3,5)\}\\
    G^S_{w,w} &= \{(1,1),(1,2),(1,3),(2,2),(2,3),(3,3)\}\\
    G^S_{b,b} &= \{(4,4),(4,5),(5,5)\}
\end{align*}
Next, consider node $u=2$, since $k=1$,
\[
    \rho(2) = \{4\}
\]
Thus, we get
\begin{align*}
    P(G^S_{w,b}) &= \frac{1}{6}\\
    P(G^S_{w,w}) &= \frac{0}{6}\\
    P(G^S_{b,b}) &= \frac{0}{3}
\end{align*}

Therefore,
\[
    \texttt{bias}(\mathcal{G}^S) = Var(\{1/6,0,0\}) = \frac{1}{162} \sim 0.006
\]

\subsubsection{Score 2: User Level}

Let $Z^S$ be the set of all possible values of attribute $S$. We calculate a bias score for an attribute value $z$ and a node $u$. 
\begin{equation}
     \texttt{bias}(z) = \frac{1}{|Z^S|} - \frac{\sum_{u \in V} \texttt{z-share}(u)}{|V|}
\end{equation}
, where 
\begin{equation}
    \texttt{z-share}(u) = \frac{|\rho_z(u)|}{|\rho(u)|} .
\end{equation}

Here, we define
\begin{equation}
    \texttt{score}_2(z,u) = \frac{1}{|Z^S|} - \texttt{z-share}(u)
\end{equation}

\noindent
Example:

Again consider the network and embedding from Figure \ref{fig:ex_1} and attribute $S=\text{race}$ with $Z^S=\{w,b\}$, $z=b$ and $k=1$.

% \note{BS: I feel it is clearer if z is a parameter of the function}
\begin{align*}
    \rho(1)&=\{2\}\\
    \rho(2)&=\{4\}\\
    \rho(3)&=\{4\}\\
    \rho(4)&=\{2\}\\
    \rho(5)&=\{2\}
\end{align*}
\begin{align*}
    \texttt{z-share}(1,b) &= \frac{0}{1}=0\\
    \texttt{z-share}(2,b) &= \frac{1}{1}=1\\
    \texttt{z-share}(3,b) &= \frac{1}{1}=1\\
    \texttt{z-share}(4,b) &= \frac{0}{1}=0\\
    \texttt{z-share}(5,b) &= \frac{0}{1}=0\\
\end{align*}
Then,
\begin{align*}
    \texttt{score}_2(z=b,u=1) &= \frac{1}{2}-\frac{0}{1}=\frac{1}{2}-0=\frac{1}{2}\\
    \texttt{score}_2(z=b,u=2) &= \frac{1}{2}-\frac{1}{1}=\frac{1}{2}-1=-\frac{1}{2}\\
    \texttt{score}_2(z=b,u=3) &= \frac{1}{2}-\frac{1}{1}=\frac{1}{2}-1=-\frac{1}{2}\\
    \texttt{score}_2(z=b,u=4) &= \frac{1}{2}-\frac{0}{1}=\frac{1}{2}-0=\frac{1}{2}\\
    \texttt{score}_2(z=b,u=5) &= \frac{1}{2}-\frac{0}{1}=\frac{1}{2}-0=\frac{1}{2}
\end{align*}
and also,
\[
\texttt{bias}(b) = \frac{1}{2} - \frac{2}{5} = \frac{1}{10} 
\]
