# Supplementary material for: BiaScope: Visual Unfairness Diagnosis for Graph Embeddings
Source: arXiv:2210.06417 source file (2022-10-12)
Supplement: Supplementary file 3 [file additional_packages.tex]

\usepackage{amsfonts}
\usepackage{amsmath}
\usepackage{hyperref}
\usepackage{xspace}
